# Supplementary material for: Lifelong Hyper-Policy Optimization with Multiple Importance Sampling Regularization
Source: arXiv:2112.06625 source file (2021-12-13)
Supplement: Supplementary file 1 [file 2_bandit_case.tex]

\section{The Bandit sub-case}
\label{app:bandit}
